# Supplementary material for: Predicting Dengue Outbreaks: A Dynamic Approach with Variable Length Markov Chains and Exogenous Factors
Source: arXiv:2410.07374 source file (2024-10-09)
Supplement: Supplementary file 1 [file material_suplementar.tex]

\documentclass[APA,Times1COL]{WileyNJDv5}
\usepackage{natbib}
\usepackage{physics}
\usepackage{gensymb}
\usepackage{threeparttable}

\usepackage{latexsym, color}
\usepackage{amsmath}
\usepackage{mathtools}
\usepackage{amsfonts}
\usepackage{amssymb}
\usepackage{psfrag}
\usepackage{graphicx}
\usepackage{epsfig}
\usepackage{multirow}
\usepackage{multicol}
\usepackage{subfigure}
\usepackage{hyperref}
\usepackage{cleveref}
\usepackage{qtree} % para desenhar arvores
\usepackage{multicol} % para colocar betas ao lado das arvores
\usepackage{tikz} % para desenhar arvores
\usepackage{forest} % para desenhar arvores
\usepackage{color}
\usepackage{calc}
\usepackage{pdfpages}

%\newcommand{\qc}{\stackrel {{\rm q.c}}{\longrightarrow}}

%\newcommand{\dd}{\stackrel {{\rm d}}{\longrightarrow}}

%% fim de   proof%%

%\DeclarePairedDelimiter\abs{\lvert}{\rvert}

\articletype{Article Type}%

\received{Date Month Year}
\revised{Date Month Year}
\accepted{Date Month Year}
\journal{Journal}
\volume{00}
\copyyear{2023}
\startpage{1}

\raggedbottom

\begin{document}

\title{Predicting Dengue Outbreaks: A Dynamic Approach with Variable Length Markov Chains and Exogenous Factors}

\author[1]{Marília Gabriela Rocha}

\author[1]{Nancy L. Garcia}

\authormark{Rocha and Garcia}
\titlemark{Predicting Dengue Outbreaks: A Dynamic Approach with Variable Length Markov Chains and Exogenous Factors}

\address[1]{\orgdiv{Statistics Department}, \orgname{Universidade Estadual de Campinas(UNICAMP)}, \orgaddress{\state{São Paulo}, \country{Brazil}}}

\corres{Corresponding author Nancy L. Garcia, Rua Sergio Buarque de Holanda, 651 - 13.083-859 - Campinas - SP - Brazil. \email{nancyg@unicamp.br}}

\presentaddress{This is sample for present address text this is sample for present address text.}

%\fundingInfo{Text}
%\JELinfo{ejlje}

\jnlcitation{\cname{%
\author{Rocha M.G.}, and
\author{Garcia N.L.}}.
\ctitle{Predicting Dengue Outbreaks.} \cjournal{\it Stat. in Medicine.} \cvol{2024;00(00):1--18}.}

%\maketitle

\section*{Supplementary Material}

\subsection*{Simulations}

In this appendix, we evaluate the performance of the proposed modified beta-context algorithm (referred to as \textit{modified-beta-VLMC} in the tables) across various scenarios, including some adapted from \citet{zanin2022variable}. The generated data follows models derived from context trees of orders 2, 3, and 4, with varying lengths of the univariate time-varying covariate parameter vector $\boldsymbol{\beta}^u$. Additionally, we explore models with and without a univariate time-invariant covariate, considering scenarios with one or more sources. For comparative analysis, in cases where the simulation involves a single source and lacks time-invariant exogenous covariates, we present results obtained using the beta-context algorithm introduced by \citet{zanin2022variable} (referred to as \textit{beta-VLMC} in the tables).

In all scenarios, the values of the tuning parameters $\delta_n$ and $f$ were selected to minimize the BIC criterion. Consequently, the same model may have different tuning parameters for the original and the modified version of the beta-context algorithm. Since tuning parameters directly affect tree length, discrepancies in tree lengths between algorithms can arise from either the algorithm itself or the tuning parameter values. However, we considered this approach better than fixing the same tuning parameters for both algorithms, as they have different constructions.

Various metrics were employed to evaluate the performance of the methods in estimating the context function. These metrics include the average values of several measures over 100 simulations:  BIC, AIC, log-likelihood, the number of parameters $\hat{\alpha}^u$ and $\hat{\boldsymbol{\gamma}}^u$ (number of final nodes $u$ in $\hat{\tau}$), the number of parameters $\hat{\boldsymbol{\beta}}^u$ (total number of coefficients estimated different from $0$ in all vectors $\hat{\boldsymbol{\beta}}^u$, $\forall u$), the order of the $\hat{\tau}$ tree, the order of the time-varying exogenous covariate (maximum length of $\hat{\boldsymbol{\beta}}^u$, $\forall u$), the number of missing nodes in $\hat{\tau}$, the number of extra nodes in $\hat{\tau}$, whether the $\tau$ tree is identified exactly (no missing and no extra nodes in $\hat{\tau}$), and whether the $\tau_{\boldsymbol{\theta}}$ tree is identified exactly (no longer nor shorter estimated parameter vector $\boldsymbol{\beta}^u$, $\forall u$). 

Furthermore, to assess the methods' performance in estimating the coefficient vector, the mean difference between real and estimated values was calculated over 100 simulations for all parameters when the context was correctly identified.

\subsection*{Simulations with a single source and without time-invariant exogenous covariates}

The simulations presented in this section were generated for a single source, and no time-invariant covariates were taken into account.  

\autoref{model1} provides details on Model 1, where time-varying exogenous variables were generated from both a standard Normal distribution (N(0, 1)) and, to evaluate performance under heavy-tailed distributions, a t-Student distribution with 2 degrees of freedom (t(2)). Samples of $n = 1000$ and $n = 2000$ state transitions were considered.

\begin{figure}[h!]
    \begin{center}
    \begin{multicols}{2}
        \noindent
        $\begin{aligned}
            \begin{forest}
            % for tree = {circle, draw, minimum size=1.5em, inner sep=2pt, s sep=3mm, l sep=7mm}
                [y 
                    [0 
                        [0(0.1) ] 
                        [1 
                            [0(0.25) ]
                            [1 
                                [0(0.8) ]
                                [1(2.0) ]]]]
                    [1 
                        [0(-0.2) ]
                        [1(-1.0) ]]]
            \end{forest}
        \end{aligned}$
        \noindent
        $\begin{aligned}
            &\boldsymbol{\beta}^{00} = (2, 0)'\\
            &\boldsymbol{\beta}^{010} = (-1, 1, 0)'\\
            &\boldsymbol{\beta}^{0111} = (1.5, 2, 0, 0)'\\
            &\boldsymbol{\beta}^{0110} = (4, 3, 2, 1)'\\
            &\boldsymbol{\beta}^{10} = (0, 0)'\\
            &\boldsymbol{\beta}^{11} = (0, 0)' 
        \end{aligned}$
    \end{multicols}
    \end{center}
    \caption{\label{model1} Context tree $\tau$ and associated parameters $\boldsymbol{\theta}$ for Model 1 (numbers in parenthesis represent the values of $\alpha^u$ for each context $u$).}
    %\legend{Source: Produced by the author}
\end{figure}

Performance metrics for both the proposed modified beta-context algorithm and the beta-context algorithm are presented in detail in \autoref{tab1-model1}. To enhance the clarity of the estimated trees, the frequency of occurrences for each context tree across 100 simulations are presented in \autoref{tab3-model1}, \autoref{tab4-model1}, \autoref{tab5-model1}, and \autoref{tab6-model1}. Each table delineates potential context trees in the first column, followed by the respective number of contexts within each tree. The last two columns indicate the frequency of occurrence for each context tree, distinguished between modified and original beta-VLMC models. Bolded lines indicate trees that were precisely estimated. 

In cases where $n = 1000$, the modifications, which require a larger number of observations to estimate exogenous covariate parameters, lead to smaller estimated trees in the proposed method compared to the real ones. Furthermore, for trees generated with exogenous time-varying covariates following a normal distribution with mean 0 and standard deviation 1, the modified version achieves a higher percentage of identical $\tau$ trees compared to the original version. However, it is important to note that both methods exhibit low accuracy.

For $n = 2000$, the modified version achieved 72\% and 83\% of identical $\tau$ trees for covariates following N(0,1) and t(2) distributions, respectively, while the original version attained 57\% and 79\%. However, the original beta-context algorithm achieved a higher percentage of identical $\tau_{\boldsymbol{\theta}}$, potentially because the modified version requires a larger number of observations to estimate covariate parameters. It is noteworthy that, in general, the original version of the beta-context algorithm generates larger trees. Both methods exhibit improved accuracy in identifying the exact same nodes as $\tau$ for $n = 2000$, supporting the consistency theory of the estimators. 

Note that even when the correct identification of $\tau_{\boldsymbol{\theta}}$ is relatively low, $\hat{\tau}$ can be correctly estimated for both methods. Yet, when the covariates are generated with a heavy-tailed t(2) distribution, the performance of both methods is not significantly affected - in fact, the accuracy of recovering $\tau_{\boldsymbol{\theta}}$ is improved.

\begin{table}[h!]
  \caption{Simulation results for Model 1 with time-varying exogenous covariates generated from N(0,1) and t(2) distributions (average over 100 simulations).}
  \label{tab1-model1}
  \centering
%\resizebox{\textwidth}{!}{%
\begin{tabular}{@{}lcc|cc@{}}
\cmidrule(l){2-5}
                                       & \multicolumn{2}{c|}{Model 1 (n = 1000, N(0, 1) distr.)} & \multicolumn{2}{c}{Model 1 (n = 1000, t(2) distr.)} \\ \cmidrule(l){2-5} 
                                       & modified-beta-VLMC              & beta-VLMC             & modified-beta-VLMC            & beta-VLMC           \\ \midrule
BIC                                    & 1154.46                         & 1153.34               & 1083.69                       & 1079.17             \\
AIC                                    & 1099.74                         & 1090.62               & 1031.69                       & 1016.86             \\
LogLik                                 & -538.72                         & -532.53               & -505.25                       & -495.73             \\
\# par. $\hat{\alpha}^u$               & 5.05                            & 5.54                  & 4.64                          & 5.19                \\
\# par. $\hat{\boldsymbol{\beta}}^u$   & 6.10                             & 7.24                  & 5.96                          & 7.50                \\
order $\hat{\tau}$                     & 3.35                            & 3.74                  & 3.25                          & 3.74                \\
order-Cov                              & 2.94                            & 3.10                   & 2.94                          & 3.37                \\
\# Missing $\hat{\tau}$                & 2.20                             & 1.95                  & 2.77                          & 2.02                \\
\# Extra $\hat{\tau}$                  & 0.30                             & 0.43                  & 0.04                          & 0.30                \\
Identical $\tau$                       & 0.16                            & 0.06                  & 0.15                          & 0.18                \\
Identical $\tau_{\boldsymbol{\theta}}$ & 0.00                               & 0.01                  & 0.00                             & 0.07                \\ \midrule
                                       & \multicolumn{2}{c|}{Model 1 (n = 2000, N(0, 1) distr.)} & \multicolumn{2}{c}{Model 1 (n = 2000, t(2) distr.)} \\ \cmidrule(l){2-5} 
                                       & modified-beta-VLMC              & beta-VLMC             & modified-beta-VLMC            & beta-VLMC           \\ \cmidrule(l){2-5} 
BIC                                    & 2252.61                         & 2260.75               & 2079.33                       & 2073.82             \\
AIC                                    & 2176.88                         & 2159.99               & 1998.40                       & 1985.44             \\
LogLik                                 & -1074.92                        & -1062.0               & -984.75                       & -976.94             \\
\# par. $\hat{\alpha}^u$               & 5.95                            & 7.15                  & 6.04                          & 6.39                \\
\# par. $\hat{\boldsymbol{\beta}}^u$   & 7.57                            & 10.84                 & 8.41                          & 9.39                \\
order $\hat{\tau}$                     & 3.85                            & 4.63                  & 3.97                          & 4.17                \\
order-Cov                              & 3.57                            & 4.07                  & 3.85                          & 3.89                \\
\# Missing $\hat{\tau}$                & 0.46                            & 0.10                   & 0.20                           & 0.10                 \\
\# Extra $\hat{\tau}$                  & 0.36                            & 2.17                  & 0.28                          & 0.78                \\
Identical $\tau$                       & 0.72                            & 0.57                  & 0.83                          & 0.79                \\
Identical $\tau_{\boldsymbol{\theta}}$ & 0.17                            & 0.30                  & 0.49                          & 0.63                \\ \bottomrule
\end{tabular}
%}
%\legend{Source: Produced by the author}
\end{table}

\begin{table}[h!]
\caption{Estimated $\tau$ trees for Model 1, with n = 1000 and N(0, 1) distribution (frequency of occurrences over 100 simulations).}
\label{tab3-model1}
\centering
%\resizebox{\textwidth}{!}{%
\begin{tabular}{lccc}
\hline
\multicolumn{1}{c}{Contexts}                        & \# Contexts & modified-beta-VLMC & beta-VLMC  \\ \hline
0 0 - 0 1 0 - 0 1 1 - 1                       & 4        & 28 & 13 \\
0 0 - 0 1 0 - 0 1 1 - 0 1 1 0 - 1             & 5        & 0  & 15 \\
0 0 - 0 1 0 - 0 1 1 - 1 0 - 1 1               & 5        & 40 & 20 \\
0 0 - 0 1 0 - 0 1 1 0 - 0 1 1 1 - 1           & 5        & 7  & 6  \\
0 0 - 0 1 0 - 0 1 1 - 0 1 1 0 - 0 1 1 0 1 - 1 & 6        & 0  & 1  \\
0 0 - 0 1 0 - 0 1 1 - 0 1 1 0 - 1 0 - 1 1     & 6        & 0  & 27 \\
0 0 - 0 1 0 - 0 1 1 - 1 0 0 - 1 0 1 - 1 1     & 6        & 1  & 1  \\
\textbf{0 0 - 0 1 0 - 0 1 1 0 - 0 1 1 1 - 1 0 - 1 1} & \textbf{6}  & \textbf{16}        & \textbf{6} \\
0 0 - 0 1 0 0 - 0 1 0 1 - 0 1 1 - 1 0 - 1 1   & 6        & 1  & 0  \\
$\geq$ 7 contexts                             & $\geq$ 7 & 7  & 11 \\ \hline
\end{tabular}%
%}
%\legend{Source: Produced by the author}
\end{table}

\begin{table}[h!]
\centering
\caption{Estimated $\tau$ trees for Model 1, with n = 1000 and t(2) distribution (frequency of occurrences over 100 simulations).}
\label{tab4-model1}
%\resizebox{\textwidth}{!}{%
\begin{tabular}{lccc}
\hline
\multicolumn{1}{c}{Contexts}                        & \# Contexts & modified-beta-VLMC & beta-VLMC   \\ \hline
0 0 - 0 1 0 - 0 1 1 - 1                           & 4 & 53 & 19 \\
0 0 - 0 1 0 - 0 1 1 - 0 1 1 0 - 1                 & 5 & 0  & 3  \\
0 0 - 0 1 0 - 0 1 1 - 1 0 - 1 1                   & 5 & 20 & 13 \\
0 0 - 0 1 0 - 0 1 1 0 - 0 1 1 1 - 1               & 5 & 9  & 34 \\
0 0 - 0 1 0 - 0 1 1 - 0 1 1 0 - 1 0 - 1 1         & 6 & 0  & 2  \\
0 0 - 0 1 0 - 0 1 1 0 - 0 1 1 0 1 - 0 1 1 1 - 1   & 6 & 0  & 1  \\
\textbf{0 0 - 0 1 0 - 0 1 1 0 - 0 1 1 1 - 1 0 - 1 1} & \textbf{6} & \textbf{15}        & \textbf{18} \\
0 0 - 0 1 0 - 0 1 1 0 0 - 0 1 1 0 1 - 0 1 1 1 - 1 & 6 & 0  & 1  \\
0 0 - 0 1 0 0 - 0 1 0 1 - 0 1 1 0 - 0 1 1 1 - 1   & 6 & 0  & 1  \\
0 0 0 - 0 0 1 - 0 1 0 - 0 1 1 - 1 0 - 1 1         & 6 & 1  & 1  \\
0 0 0 - 0 0 1 - 0 1 0 - 0 1 1 0 - 0 1 1 1 - 1     & 6 & 1  & 1  \\
$\geq$ 7 contexts                                     & 7 & 0  & 5  \\ \hline
\end{tabular}%
%}
%\legend{Source: Produced by the author}
\end{table}

\begin{table}[h!]
\caption{Estimated $\tau$ trees for Model 1, with n = 2000 and N(0, 1) distribution (frequency of occurrences over 100 simulations).}
\label{tab5-model1}
\centering
%\resizebox{\textwidth}{!}{%
\begin{tabular}{lccc}
\hline
\multicolumn{1}{c}{Contexts}               & \# Contexts & modified-beta-VLMC & beta-VLMC \\ \hline
0 0 - 0 1 0 - 0 1 1 - 1 0 - 1 1             & 5           & 22                 & 3         \\
\textbf{0 0 - 0 1 0 - 0 1 1 0 - 0 1 1 1 - 1 0 - 1 1} & \textbf{6}           & \textbf{72}                 & \textbf{57}        \\
$\geq 7$ contexts                  & $\geq 7$           & 6                  & 40        \\ \hline
\end{tabular}%
%}
%\legend{Source: Produced by the author}
\end{table}

\begin{table}[h!]
\caption{Estimated $\tau$ trees for Model 1, with n = 2000 and t(2) distribution (frequency of occurrences over 100 simulations).}
\label{tab6-model1}
\centering
%\resizebox{\textwidth}{!}{%
\begin{tabular}{lccc}
\hline
\multicolumn{1}{c}{Contexts}               & \# Contexts & modified-beta-VLMC & beta-VLMC \\ \hline
0 0 - 0 1 0 - 0 1 1 - 1 0 - 1 1             & 5           & 6                  & 1         \\
0 0 - 0 1 0 - 0 1 1 0 - 0 1 1 1 - 1         & 5           & 4                  & 3         \\
\textbf{0 0 - 0 1 0 - 0 1 1 0 - 0 1 1 1 - 1 0 - 1 1} & \textbf{6}           & \textbf{83}                 & \textbf{79}        \\
$\geq 7$ contexts                  & $\geq 7$          & 7                  & 17        \\ \hline
\end{tabular}%
%}
%\legend{Source: Produced by the author}
\end{table}

To evaluate the performance of the proposed method in estimating the vector of coefficients, \autoref{tab2-model1} presents the mean differences between real and estimated parameters for both the modified and original beta-context algorithms when the context is correctly identified. For parameters corresponding to short contexts, such as $u = (0, 0)$, estimation accuracy is high for both methods. However, larger contexts like (0,1,1,0) and (0,1,1,1) were infrequent in the data generated by Model 1, especially for $n = 1000$, leading to insufficient observations for accurate estimation of these six parameters. Generally, when the context is present in the final tree, the modified version provides better estimates.

\begin{table}[h!]
\centering
\caption{Differences between real and estimated values for Model 1 (average over 100 simulations).}
\label{tab2-model1}
%\resizebox{\textwidth}{!}{%
\begin{tabular}{lcc|cc}
\cline{2-5}
                            & \multicolumn{2}{c|}{Model 1 (n = 1000, N(0, 1) distr.)} & \multicolumn{2}{c}{Model 1 (n = 1000, t(2) distr.)} \\ \cline{2-5} 
                            & modified-beta-VLMC         & beta-VLMC                  & modified-beta-VLMC       & beta-VLMC                \\ \hline
$\alpha^{00}$               & 0.14                       & 0.14                       & 0.14                     & 0.14                     \\
$\alpha^{010}$              & 0.14                       & 0.14                       & 0.18                     & 1.18                     \\
$\alpha^{0110}$             & 0.68                       & 1.34                       & 2.11                     & 1.83                     \\
$\alpha^{0111}$             & 0.81                       & 0.81                       & 1.07                     & 4.16                     \\
$\alpha^{10}$               & 0.08                       & 0.08                       & 0.09                     & 0.09                     \\
$\alpha^{11}$               & 0.13                       & 0.13                       & 0.14                     & 0.15                     \\
$\boldsymbol{\beta}^{00}$   & (0.26, 0)                  & (0.26, 0)                  & (0.26, 0)                & (0.25, 0)                \\
$\boldsymbol{\beta}^{010}$  & (0.16, 0.22, 0)            & (0.16, 0.22, 0)            & (0.18, 0.18, 0)          & (0.18, 0.18, 0)          \\
$\boldsymbol{\beta}^{0110}$ & (1.50, 2.00, 0, 0)         & (1.10, 1.53, 0, 0)         & (1.50, 2.00, 0, 0)       & (4.65, 4.88, 1.17, 0)    \\
$\boldsymbol{\beta}^{0111}$ & (2.10, 1.88, 1.38, 1.42)   & (2.89, 2.40, 1.51, 1.54)   & (9.14, 7.82, 5.11, 2.49) & (7.39, 5.82, 3.87, 2.27) \\
$\boldsymbol{\beta}^{10}$   & (0, 0)                     & (0, 0)                     & (0, 0)                   & (0, 0)                   \\
$\boldsymbol{\beta}^{11}$   & (0, 0)                     & (0, 0)                     & (0,0)                    & (0, 0)                   \\ \hline
                            & \multicolumn{2}{c|}{Model 1 (n = 2000, N(0, 1) distr.)} & \multicolumn{2}{c}{Model 1 (n = 2000, t(2) distr.)} \\ \cline{2-5} 
                            & modified-beta-VLMC         & beta-VLMC                  & modified-beta-VLMC       & beta-VLMC                \\ \hline
$\alpha^{00}$               & 0.10                       & 0.10                       & 0.09                     & 0.09                     \\
$\alpha^{010}$              & 0.10                       & 0.10                       & 0.12                     & 0.12                     \\
$\alpha^{0110}$             & 0.28                       & 0.27                       & 0.38                     & 0.37                     \\
$\alpha^{0111}$             & 0.66                       & 1.14                       & 0.69                     & 1.03                     \\
$\alpha^{10}$               & 0.06                       & 0.06                       & 0.06                     & 0.06                     \\
$\alpha^{11}$               & 0.08                       & 0.08                       & 0.09                     & 0.09                     \\
$\boldsymbol{\beta}^{00}$   & (0.16, 0)                  & (0.16, 0)                  & (0.16, 0)                & (0.15, 0)                \\
$\boldsymbol{\beta}^{010}$  & (0.13, 0.12, 0)            & (0.13, 0.12, 0)            & (0.13, 0.15, 0)          & (0.13, 0.15, 0)          \\
$\boldsymbol{\beta}^{0110}$ & (0.10, 1.28, 0, 0)         & (0.63, 1.36, 0.32, 0.31)   & (0.82, 1.09, 0, 0)       & (0.82, 1.32, 0, 0)       \\
$\boldsymbol{\beta}^{0111}$ & (0.75, 0.58, 0.47, 0.63)   & (0.76, 0.56, 0.45, 0.71)   & (0.98, 0.72, 0.49, 0.41) & (0.96, 0.70, 0.48, 0.44) \\
$\boldsymbol{\beta}^{10}$   & (0, 0)                     & (0, 0)                     & (0, 0)                   & (0, 0)                   \\
$\boldsymbol{\beta}^{11}$   & (0, 0)                     & (0, 0)                     & (0, 0)                   & (0, 0)                   \\ \hline
\end{tabular}%
%}
\end{table}

Model 2 is described in \autoref{model2} and involves generating time-varying exogenous covariates from a N(0, 1) distribution. We create samples with $n=1000$ and $n=2000$ state transitions.

\begin{figure}[h!]
    \begin{center}
    \begin{multicols}{2}
        \noindent
        $\begin{aligned}
            \begin{forest}
            % for tree = {circle, draw, minimum size=1.5em, inner sep=2pt, s sep=3mm, l sep=7mm}
                [y 
                    [0 
                        [0 
                            [0(0.5)]
                            [1(0.8)]] 
                        [1(1.0) ]]
                    [1 
                        [0(-0.2) ]
                        [1(0.5) ]]]
            \end{forest}
        \end{aligned}$
        \noindent
        $\begin{aligned}
            &\boldsymbol{\beta}^{000} = (3, 1, 2)'\\
            &\boldsymbol{\beta}^{001} = (1, 0, 0)'\\
            &\boldsymbol{\beta}^{01} = (-1, -2)'\\
            &\boldsymbol{\beta}^{10} = (-1.2, 0)'\\
            &\boldsymbol{\beta}^{11} = (0, 0)' 
        \end{aligned}$
    \end{multicols}
    \end{center}
    \caption{\label{model2} Context tree $\tau$ and associated parameters $\boldsymbol{\theta}$ for Model 2 (numbers in parenthesis represent the values of $\alpha^u$ for each context $u$).}
   % \legend{Source: Produced by the author}
\end{figure}

The performance metrics for the estimated context function in Model 2 are detailed in \autoref{tab1-model2}. To aid in the visualization of the estimated trees, \autoref{tab3-model2} and \autoref{tab4-model2} provide the count of estimated occurrences for each context. In both instances with $n = 1000$ and $n = 2000$, the modified beta-VLMC algorithm demonstrated a superior percentage of identical $\tau$ trees and exact covariate vectors $\tau_{\boldsymbol{\theta}}$ when compared to the original algorithm introduced by \citet{zanin2022variable}. It is noteworthy that, overall, the original algorithm tends to produce larger trees. Both methods fit better Model 2 than Model 1, either by under or overfitting, probably because it has a larger sample size when compared to the number of parameters to be estimated. 

\begin{table}[h!]
 \caption{Simulation results for Model 2 with time-varying exogenous covariates generated from a N(0, 1) distribution (average over 100 simulations).}
  \label{tab1-model2}
  \centering
%\resizebox{\textwidth}{!}{%
\begin{tabular}{lcc|cc}
\cline{2-5}
                                       & \multicolumn{2}{c|}{Model 2 (n = 1000, N(0, 1) distr.)} & \multicolumn{2}{c}{Model 2 (n = 2000, N(0, 1) distr.)} \\ \cline{2-5} 
                                       & modified-beta-VLMC              & beta-VLMC             & modified-beta-VLMC             & beta-VLMC             \\ \hline
BIC                                    & 1160.27                         & 1183.37               & 2261.52                        & 2264.89               \\
AIC                                    & 1108.0                          & 1118.47               & 2185.40                        & 2183.90               \\
logLik                                 & -543.35                         & -545.31               & -1079.03                       & -1077.49              \\
\# par. $\hat{\alpha}^u$               & 4.77                            & 5.89                  & 5.50                            & 5.76                  \\
\# par. $\hat{\boldsymbol{\beta}}^u$   & 5.88                            & 7.37                  & 8.09                           & 8.70                   \\
order $\hat{\tau}$                     & 2.79                            & 3.64                  & 3.37                           & 3.49                  \\
order-Cov                              & 2.76                            & 3.53                  & 3.32                           & 3.23                  \\
\# Missing $\hat{\tau}$                & 0.50                             & 0.44                  & 0                              & 0                     \\
\# Extra $\hat{\tau}$                  & 0.04                            & 2.09                  & 1.00                              & 1.40                   \\
Identical $\tau$                       & 0.76                            & 0.58                  & 0.87                           & 0.76                  \\
Identical $\tau_{\boldsymbol{\theta}}$ & 0.35                            & 0.29                  & 0.86                           & 0.76                  \\ \hline
\end{tabular}%
%}
%\legend{Source: Produced by the author}
\end{table}

\begin{table}[h!]
\caption{Estimated $\tau$ trees for Model 2, with n = 1000 (frequency of occurrences over 100 simulations).}
\label{tab3-model2}
\centering
%\resizebox{\textwidth}{!}{%
\begin{tabular}{lccc}
\hline
\multicolumn{1}{c}{Contexts}               & \# Contexts & modified-beta-VLMC & beta-VLMC \\ \hline
0 0 - 0 1 - 1                               & 3           & 1                  & 1         \\
0 0 - 0 1 - 1 0 - 1 1                       & 4           & 21                 & 16        \\
0 0 0 - 0 0 1 - 0 1 - 1                     & 4           & 1                  & 1         \\
\textbf{0 0 0 - 0 0 1 - 0 1 - 1 0 - 1 1}             & \textbf{5}           & \textbf{76}                 & \textbf{58}        \\
0 0 - 0 1 0 - 0 1 1 0 - 0 1 1 1 - 1 0 - 1 1 & 6           & 1                  & 0         \\
\textgreater{}= 7 contexts                  & 7           & 0                  & 24        \\ \hline
\end{tabular}%
%}
%\legend{Source: Produced by the author}
\end{table}

\begin{table}[h!]
\caption{Estimated $\tau$ trees for Model 2, with n = 2000 (frequency of occurrences over 100 simulations).}
\label{tab4-model2}
\centering
%\resizebox{\textwidth}{!}{%
\begin{tabular}{lccc}
\hline
\multicolumn{1}{c}{Contexts}               & \# Contexts & modified-beta-VLMC & beta-VLMC \\ \hline
\textbf{0 0 0 - 0 0 1 - 0 1 - 1 0 - 1 1}             & \textbf{5}           & \textbf{87}                 & \textbf{76}        \\
0 0 0 0 - 0 0 0 1 - 0 0 1 - 0 1 - 1 0 - 1 1 & 6           & 0                  & 2         \\
\textgreater{}= 7 contexts                  & 7           & 13                 & 22        \\ \hline
\end{tabular}%
%}
%\legend{Source: Produced by the author}
\end{table}

\autoref{tab2-model2} shows the mean differences between real and estimated parameters for both the modified and original beta-context algorithms when the context is correctly identified. Overall, both methods yield comparable results.

\begin{table}[h!]
\caption{Differences between real and estimated values for Model 2 (average over 100 simulations).}
\label{tab2-model2}
\centering
%\resizebox{\textwidth}{!}{%
\begin{tabular}{lcc|cc}
\cline{2-5}
                           & \multicolumn{2}{c|}{Model 2 (n = 1000, N(0, 1) distr.)} & \multicolumn{2}{c}{Model 2 (n = 2000, N(0,1) distr.)} \\ \cline{2-5} 
                           & modified-beta-VLMC         & beta-VLMC                  & modified-beta-VLMC        & beta-VLMC                 \\ \hline
$\alpha^{000}$             & 0.57                       & 0.56                       & 0.28                      & 0.28                      \\
$\alpha^{001}$             & 0.19                       & 0.19                       & 0.15                      & 0.15                      \\
$\alpha^{01}$              & 0.17                       & 0.17                       & 0.11                      & 0.10                      \\
$\alpha^{10}$              & 0.12                       & 0.12                       & 0.08                      & 0.08                      \\
$\alpha^{11}$              & 0.09                       & 0.09                       & 0.06                      & 0.06                      \\
$\boldsymbol{\beta}^{000}$ & (1.02, 0.66, 0.84)         & (1.04, 0.67, 0.87)         & (0.54, 0.27, 0.37)        & (0.53, 0.26, 0.36)        \\
$\boldsymbol{\beta}^{001}$ & (0.66, 0, 0)               & (0.65, 0, 0)               & (0.17, 0, 0)              & (0.16, 0, 0)              \\
$\boldsymbol{\beta}^{01}$  & (0.17, 0.21)               & (0.18, 0.22)               & (0.10, 0.15)              & (0.10, 0.15)              \\
$\boldsymbol{\beta}^{10}$  & (0.15, 0)                  & (0.16, 0)                  & (0.10, 0)                 & (0.10, 0)                 \\
$\boldsymbol{\beta}^{11}$  & (0,0)                      & (0,0)                      & (0,0)                     & (0,0)                     \\ \hline
\end{tabular}%
%}
%\legend{Source: Produced by the author}
\end{table}

In Model 3, as outlined in \autoref{model3}, we assess the effectiveness of the proposed algorithm when data is generated from a full tree of fixed order. Time-varying exogenous variables were generated from a N(0,1) distribution. We generate samples with $n = 1000$ and $n = 2000$ state transitions.

\begin{figure}[h!]
    \begin{center}
    \begin{multicols}{2}
        \noindent
        $\begin{aligned}
            \begin{forest}
            % for tree = {circle, draw, minimum size=1.5em, inner sep=2pt, s sep=3mm, l sep=7mm}
                [y 
                    [0 
                        [0(0.1) ] 
                        [1(0.25) ]]
                    [1 
                        [0(1.0) ]
                        [1(0.8) ]]]
            \end{forest}
        \end{aligned}$
        \noindent
        $\begin{aligned}
            &\boldsymbol{\beta}^{00} = (1.2, 0.3)'\\
            &\boldsymbol{\beta}^{01} = (-1, 1)'\\
            &\boldsymbol{\beta}^{10} = (1.5, -2)'\\
            &\boldsymbol{\beta}^{11} = (-0.2, -0.9)' 
        \end{aligned}$
    \end{multicols}
    \end{center}
    \caption{\label{model3} Context tree $\tau$ and associated parameters $\boldsymbol{\theta}$ for Model 3 (numbers in parenthesis represent the values of $\alpha^u$ for each context $u$).}
    %\legend{Source: Produced by the author}
\end{figure}

The performance metrics for the estimated context function in Model 3 are outlined in \autoref{tab1-model3}. To aid in the visualization of the estimated trees, \autoref{tab3-model3} and \autoref{tab4-model3} provide the count of estimated occurrences for each context. For $n = 1000$, the original beta-context algorithm demonstrated superior results, achieving 100\% identical $\tau$ trees, while the modified beta-context algorithm produced larger trees than the real ones. For $n = 2000$, improved outcomes were observed with the modified beta-context algorithm. Interestingly, in this case, the original beta-context algorithm generated larger trees than the real ones - 23 trees with more than seven contexts when the real tree has only 4 contexts. 

\begin{table}[h!]
\caption{Simulation results for Model 3 with time-varying exogenous covariates generated from a N(0, 1) distribution (average over 100 simulations).}
  \label{tab1-model3}
  \centering
%\resizebox{\textwidth}{!}{%
\begin{tabular}{lcc|cc}
\cline{2-5}
                                       & \multicolumn{2}{c|}{Model 3 (n = 1000, N(0, 1) distr.)} & \multicolumn{2}{c}{Model 3 (n = 2000, N(0, 1) distr.)} \\ \cline{2-5} 
                                       & modified-beta-VLMC              & beta-VLMC             & modified-beta-VLMC             & beta-VLMC             \\ \hline
BIC                                    & 1123.18                         & 1120.03               & 2184.90                        & 2195.48               \\
AIC                                    & 1065.71                        & 1066.29               & 2116.06                        & 2115.72               \\
logLik                                 & -521.15                         & -522.19               & -1045.74                       & -1043.62              \\
\# par. $\hat{\alpha}^u$               & 4.25                            & 4.00                     & 4.36                           & 4.99                  \\
\# par. $\hat{\boldsymbol{\beta}}^u$   & 7.46                            & 6.95                  & 7.93                           & 9.25                  \\
order $\hat{\tau}$                     & 2.25                            & 2.00                     & 2.36                           & 2.93                  \\
order-Cov                              & 2.23                            & 2.00                     & 2.25                           & 2.56                  \\
\# Missing $\hat{\tau}$                & 0                               & 0                     & 0                              & 0                     \\
\# Extra $\hat{\tau}$                  & 0.50                             & 0                     & 0.72                           & 1.78                  \\
Identical $\tau$                       & 0.90                             & 1.00                     & 0.86                           & 0.71                  \\
Identical $\tau_{\boldsymbol{\theta}}$ & 0                               & 0                     & 0.13                           & 0.11                  \\ \hline
\end{tabular}%
%}
%\legend{Source: Produced by the author}
\end{table}

\begin{table}[h!]
\caption{Estimated $\tau$ trees for Model 3, with n = 1000 (frequency of occurrences over 100 simulations).}
\label{tab3-model3}
\centering
%\resizebox{\textwidth}{!}{%
\begin{tabular}{lccc}
\hline
\multicolumn{1}{c}{Contexts}                & \# Contexts & modified-beta-VLMC & beta-VLMC \\ \hline
\textbf{0 0 - 0 1 - 1 0 - 1 1}                       & \textbf{4}           & \textbf{90}                 & \textbf{100}       \\
0 0 - 0 1 - 1 0 - 1 1 0 - 1 1 1             & 5           & 1                  & 0         \\
0 0 - 0 1 - 1 0 0 - 1 0 1 0 - 1 0 1 1 - 1 1 & 6           & 1                  & 0         \\
0 0 - 0 1 0 0 - 0 1 0 1 - 0 1 1 - 1 0 - 1 1 & 6           & 1                  & 0         \\
0 0 0 0 - 0 0 0 1 - 0 0 1 - 0 1 - 1 0 - 1 1 & 6           & 1                  & 0         \\
\textgreater{}= 7 contexts                  & 7           & 6                  & 0  \\ \hline      
\end{tabular}%
%}
%\legend{Source: Produced by the author}
\end{table}

\begin{table}[h!]
\caption{Estimated $\tau$ trees for Model 3, with n = 2000 (frequency of occurrences over 100 simulations).}
\label{tab4-model3}
\centering
%\resizebox{\textwidth}{!}{%
\begin{tabular}{lccc}
\hline
\multicolumn{1}{c}{Contexts}               & \# Contexts & modified-beta-VLMC & beta-VLMC \\ \hline
\textbf{0 0 - 0 1 - 1 0 - 1 1}                       & \textbf{4}           & \textbf{86}                 & \textbf{71}        \\
0 0 - 0 1 - 1 0 0 - 1 0 1 - 1 1             & 5           & 2                  & 1         \\
0 0 - 0 1 0 - 0 1 1 - 1 0 - 1 1             & 5           & 1                  & 1         \\
0 0 - 0 1 - 1 0 - 1 1 0 0 - 1 1 0 1 - 1 1 1 & 6           & 1                  & 1         \\
0 0 - 0 1 - 1 0 0 - 1 0 1 0 - 1 0 1 1 - 1 1 & 6           & 1                  & 3         \\
0 0 - 0 1 - 1 0 0 0 - 1 0 0 1 - 1 0 1 - 1 1 & 6           & 1                  & 0         \\
\textgreater{}= 7 contexts                  & 7           & 8                  & 23        \\ \hline
\end{tabular}%
%}
%\legend{Source: Produced by the author}
\end{table}

The mean discrepancies between real and estimated parameters, when the context was correctly identified, are shown in \autoref{tab2-model3} for both the proposed modified beta-context algorithm and the beta-context algorithm. Both methods exhibit comparable results in this scenario.

\begin{table}[h!]
\caption{Differences between real and estimated values for Model 3 (average over 100 simulations).}
\label{tab2-model3}
\centering
%\resizebox{\textwidth}{!}{%
\begin{tabular}{lcc|cc}
\cline{2-5}
                          & \multicolumn{2}{c|}{Model 3 (n = 1000, N(0, 1) distr.)} & \multicolumn{2}{c}{Model 3 (n = 2000, N(0,1) distr.)} \\ \cline{2-5} 
                          & modified-beta-VLMC            & beta-VLMC               & modified-beta-VLMC           & beta-VLMC              \\ \hline
$\alpha^{00}$             & 0.13                          & 0.13                    & 0.10                          & 0.10                    \\
$\alpha^{01}$             & 0.13                          & 0.14                    & 0.09                         & 0.09                   \\
$\alpha^{10}$             & 0.18                          & 0.18                    & 0.13                         & 0.13                   \\
$\alpha^{11}$             & 0.11                          & 0.11                    & 0.07                         & 0.07                   \\
$\boldsymbol{\beta}^{00}$ & (0.15, 0.3)                   & (0.16, 0.3)             & (0.13, 0.27)                 & (0.14, 0.27)           \\
$\boldsymbol{\beta}^{01}$ & (0.15, 0.15)                  & (0.15, 0.17)            & (0.10, 0.11)                 & (0.10, 0.11)           \\
$\boldsymbol{\beta}^{10}$ & (0.23, 0.26)                  & (0.23, 0.25)            & (0.15, 0.15)                 & (0.15, 0.15)           \\
$\boldsymbol{\beta}^{11}$ & (0.10, 0.11)                  & (0.10, 0.12)            & (0.07, 0.08)                 & (0.06, 0.08)           \\ \hline
\end{tabular}%
%}
%\legend{Source: Produced by the author}
\end{table}

%\autoref{tab3-model3} and \autoref{tab4-model3} present the estimated contexts for each simulation. It is noteworthy that for $n = 2000$, the original beta-context algorithm generates 23 trees with more than seven contexts when the real tree has only 4 contexts. However, for $n = 1000$, the original beta-context algorithm produces 100\% identical trees.

In Model 4, as outlined in \autoref{model4}, we evaluate the effectiveness of the proposed algorithm in situations where the state space is not binary. Time-varying exogenous variables were generated from a N(0,1) distribution. Given its larger number of parameters to be estimated, we generate samples with $n = 4000$ and $n = 8000$ state transitions.

\begin{figure}[h!]
    \begin{center}
        \begin{forest}
        % for tree = {circle, draw, minimum size=1.5em, inner sep=2pt, s sep=3mm, l sep=7mm}
            [y 
                [0 
                    [0(-0.3;0.6) ] 
                    [1(-0.5;-0.5) ] 
                    [2(-0.35;-1.0) ]]
                [1(0.2;-0.2) 
                    [0(-0.2;0.7) ]]
                [2(1.0;-1.3) ]]
        \end{forest}
        \begin{multicols}{2}
            \noindent
            $\begin{aligned}
                &\boldsymbol{\beta}^{00}_1 = (0.4, 0)'\\
                &\boldsymbol{\beta}^{01}_1 = (0.9, 0)'\\
                &\boldsymbol{\beta}^{02}_1 = (1.5, -2)'\\
                &\boldsymbol{\beta}^{10}_1 = (0, 0)' \\
                &\boldsymbol{\beta}^{1*}_1 = (-0.4)' \\
                &\boldsymbol{\beta}^{2}_1 = (0)'
            \end{aligned}$
            \noindent
            $\begin{aligned}
                &\boldsymbol{\beta}^{00}_2 = (0.4, 0)'\\
                &\boldsymbol{\beta}^{01}_2 = (0.3, 0)'\\
                &\boldsymbol{\beta}^{02}_2 = (0.5, -0.85)'\\
                &\boldsymbol{\beta}^{10}_2 = (0, 0)' \\
                &\boldsymbol{\beta}^{1*}_2 = (0.6)' \\
                &\boldsymbol{\beta}^{2}_2 = (0)' 
            \end{aligned}$
        \end{multicols}
    \end{center}
    \caption{\label{model4} Context tree $\tau$ and associated parameters $\boldsymbol{\theta}$ for Model 4. Numbers in parenthesis represent the values of $(\alpha_1^u, \alpha_2^u)$ from each context $u$ and $\boldsymbol{\beta}_1^u$ and $\boldsymbol{\beta}_2^u$ are the coefficient vectors of the covariates. $\boldsymbol{\beta}^{1*}$ means the context is 1 preceded by other states that are not 1.}
   % \legend{Source: Produced by the author}
\end{figure}

The performance metrics for the estimated context function in Model 4 are detailed in \autoref{tab1-model4}. To aid in the visualization of the estimated trees, \autoref{tab3-model4} and \autoref{tab4-model4} provide the count of estimated occurrences for each context. For $n = 4000$, both algorithms yielded similar results, with the original beta-context algorithm having a higher percentage of identical $\tau$ trees (98\% compared to 95\% for the modified beta-context algorithm) but a lower percentage of exact covariate vectors (24\% compared to 38\% for the modified beta-context algorithm). For $n = 8000$, the modified beta-context algorithm demonstrated superior results, achieving 100\% and 76\% identical $\tau$ trees and exact covariate vectors, respectively. Both methods showed better results in achieving exact covariate vectors with $n = 8000$. In general, the original beta-context algorithm resulted in larger trees.

\begin{table}[h!]
\centering
\caption{Simulation results for Model 4 with time-varying exogenous covariates generated from a N(0, 1) distribution (average over 100 simulations).}
\label{tab1-model4}
%\resizebox{\textwidth}{!}{%
\begin{tabular}{lcc|cc}
\cline{2-5}
 & \multicolumn{2}{c|}{Model 4 (n = 4000, N(0, 1) distr.)} & \multicolumn{2}{c}{Model 4 (n = 8000, N(0, 1) distr.)} \\ \cline{2-5} 
                                       & modified-beta-VLMC & beta-VLMC & modified-beta-VLMC & beta-VLMC \\ \hline
BIC                                    & 7661.21            & 7658.67   & 15160.71           & 15189.83  \\
AIC                                    & 7526.39            & 7527.75   & 15010.34           & 15008.16  \\
logLik                                 & -3741.78           & -3743.08  & -7483.65           & -7478.08  \\
\# par. $\hat{\alpha}^u$                & 12.32              & 12.14     & 12                 & 14.04     \\
\# par. $\hat{\boldsymbol{\beta}}^u$    & 9.10               & 8.66      & 9.52               & 11.96     \\
order $\hat{\tau}$                     & 2.14               & 2.06      & 2                  & 2.67      \\
order-Cov                              & 2.05               & 2.05      & 2                  & 2.4       \\
\# Missing $\hat{\tau}$                 & 0                  & 0         & 0                  & 0         \\
\# Extra $\hat{\tau}$                   & 0.18               & 0.07      & 0                  & 1.08      \\
Identical $\tau$                       & 0.95               & 0.98      & 1                  & 0.79      \\
Identical $\tau_{\boldsymbol{\theta}}$ & 0.38               & 0.24      & 0.76               & 0.70      \\ \hline
\end{tabular}%
%}
%\legend{Source: Produced by the author}
\end{table}

\begin{table}[]
\centering
\caption{Estimated $\tau$ trees for Model 4, with n = 4000 (frequency of occurrences over 100 simulations).}
\label{tab3-model4}
%\resizebox{\textwidth}{!}{
\begin{tabular}{lccc}
\hline
\multicolumn{1}{c}{Contexts}                               & \# Contexts & modified-beta-VLMC & beta-VLMC \\ \hline
\textbf{0 0 - 0 1 - 0 2 - 1 - 1 0 - 2}                               & \textbf{6}          & \textbf{95}                 & \textbf{98}        \\
0 0 - 0 0 2 - 0 0 2 0 - 0 1 - 0 2 - 1 - 1 0 - 2             & 8          & 1                  & 0         \\
0 0 - 0 1 - 0 1 1 - 0 1 1 1 - 0 2 - 1 - 1 0 - 2             & 8          & 1                  & 0         \\
0 0 - 0 0 1 - 0 0 1 1 - 0 0 1 1 2 - 0 1 - 0 2 - 1 - 1 0 - 2 & 9          & 0                  & 1         \\
$\geq$ 10 contexts                                              & 10         & 3                  & 1         \\ \hline
\end{tabular}%
%}
%\legend{Source: Produced by the author}
\end{table}

\begin{table}[]
\centering
\caption{Estimated $\tau$ trees for Model 4, with n = 8000 (frequency of occurrences over 100 simulations).}
\label{tab4-model4}
%\resizebox{\textwidth}{!}{%
\begin{tabular}{lccc}
\hline
\multicolumn{1}{c}{Contexts}                               & \# Contexts & modified-beta-VLMC & beta-VLMC \\ \hline
\textbf{0 0 - 0 1 - 0 2 - 1 - 1 0 - 2}                               & \textbf{6}          & \textbf{100}                & \textbf{79}        \\
0 0 - 0 0 0 - 0 0 0 1 - 0 0 0 1 2 - 0 1 - 0 2 - 1 - 1 0 - 2 & 9          & 0                  & 1         \\
0 0 - 0 0 1 - 0 0 1 1 - 0 0 1 1 2 - 0 1 - 0 2 - 1 - 1 0 - 2 & 9          & 0                  & 1         \\
0 0 - 0 0 2 - 0 0 2 1 - 0 0 2 1 0 - 0 1 - 0 2 - 1 - 1 0 - 2 & 9          & 0                  & 1         \\
0 0 - 0 1 - 0 1 1 - 0 1 1 2 - 0 1 1 2 0 - 0 2 - 1 - 1 0 - 2 & 9          & 0                  & 2         \\
0 0 - 0 1 - 0 1 1 - 0 1 1 2 - 0 1 1 2 1 - 0 2 - 1 - 1 0 - 2 & 9          & 0                  & 1         \\
0 0 - 0 1 - 0 1 2 - 0 1 2 1 - 0 1 2 1 0 - 0 2 - 1 - 1 0 - 2 & 9          & 0                  & 1         \\
0 0 - 0 1 - 0 2 - 0 2 1 - 0 2 1 1 - 0 2 1 1 1 - 1 - 1 0 - 2 & 9          & 0                  & 1         \\
0 0 - 0 1 - 0 2 - 1 - 1 0 - 2 - 2 0 - 2 0 0 - 2 0 0 2       & 9          & 0                  & 1         \\
0 0 - 0 1 - 0 2 - 1 - 1 0 - 2 - 2 0 - 2 0 1 - 2 0 1 0       & 9          & 0                  & 1         \\
$\geq$ 10 contexts                                              & 10         & 0                  & 11        \\ \hline
\end{tabular}%
%}
%\legend{Source: Produced by the author}
\end{table}

The mean discrepancies between real and estimated parameters, when the context was correctly identified, are shown in \autoref{tab2-model4}. Both methods exhibit comparable results in this scenario.

\begin{table}[h!]
\centering
\caption{Differences between real and estimated values for Model 4 (average over 100 simulations).}
\label{tab2-model4}
%\resizebox{\textwidth}{!}{%
\begin{tabular}{lcc|cc}
\cline{2-5}
 &
  \multicolumn{2}{c|}{Model 4 (n = 4000, N(0, 1) distr.)} &
  \multicolumn{2}{c}{Model 4 (n = 8000, N(0,1) distr.)} \\ \cline{2-5} 
 &
  modified-beta-VLMC &
  beta-VLMC &
  modified-beta-VLMC &
  beta-VLMC \\ \hline
($\alpha^{00}_1$, $\alpha^{00}_2$) &
  (0.09, 0.08) &
  (0.09, 0.08) &
  (0.09, 0.07) &
  (0.09, 0.07) \\
($\alpha^{01}_1$, $\alpha^{01}_2$) &
  (0.09, 0.09) &
  (0.09, 0.09) &
  (0.06, 0.05) &
  (0.07, 0.05) \\
($\alpha^{02}_1$, $\alpha^{02}_2$) &
  (0.15, 0.20) &
  (0.15, 0.20) &
  (0.10, 0.13) &
  (0.10, 0.13) \\
($\alpha^{10}_1$, $\alpha^{10}_2$) &
  (0.13, 0.11) &
  (0.13, 0.11) &
  (0.09, 0.07) &
  (0.09, 0.07) \\
($\alpha^{1*}_1$, $\alpha^{1*}_2$) &
  (0.05, 0.06) &
  (0.06, 0.06) &
  (0.04, 0.04) &
  (0.04, 0.04) \\
($\alpha^{2}_1$, $\alpha^{2}_2$) &
  (0.06, 0.09) &
  (0.06, 0.09) &
  (0.04, 0.06) &
  (0.04, 0.07) \\
\begin{tabular}[c]{@{}l@{}}$\boldsymbol{\beta}^{00}_1$\\ $\boldsymbol{\beta}^{00}_2$\end{tabular} &
  \begin{tabular}[c]{@{}c@{}}(0.29, 0)\\ (0.28, 0)\end{tabular} &
  \begin{tabular}[c]{@{}c@{}}(0.34, 0)\\ (0.34, 0)\end{tabular} &
  \begin{tabular}[c]{@{}c@{}}(0.16, 0)\\ (0.15, 0)\end{tabular} &
  \begin{tabular}[c]{@{}c@{}}(0.12, 0)\\ (0.11, 0)\end{tabular} \\
\begin{tabular}[c]{@{}l@{}}$\boldsymbol{\beta}^{01}_1$\\ $\boldsymbol{\beta}^{01}_2$\end{tabular} &
  \begin{tabular}[c]{@{}c@{}}(0.10, 0)\\ (0.09, 0)\end{tabular} &
  \begin{tabular}[c]{@{}c@{}}(0.10, 0)\\ (0.09, 0)\end{tabular} &
  \begin{tabular}[c]{@{}c@{}}(0.08, 0)\\ (0.07, 0)\end{tabular} &
  \begin{tabular}[c]{@{}c@{}}(0.08, 0)\\ (0.07, 0)\end{tabular} \\
\begin{tabular}[c]{@{}l@{}}$\boldsymbol{\beta}^{02}_1$\\ $\boldsymbol{\beta}^{02}_2$\end{tabular} &
  \begin{tabular}[c]{@{}c@{}}(0.19, 0.22)\\ (0.19, 0.20)\end{tabular} &
  \begin{tabular}[c]{@{}c@{}}(0.19, 0.22)\\ (0.19, 0.19)\end{tabular} &
  \begin{tabular}[c]{@{}c@{}}(0.13, 0.19)\\ (0.14, 0.15)\end{tabular} &
  \begin{tabular}[c]{@{}c@{}}(0.13, 0.18)\\ (0.13, 0.15)\end{tabular} \\
\begin{tabular}[c]{@{}l@{}}$\boldsymbol{\beta}^{10}_1$\\ $\boldsymbol{\beta}^{10}_2$\end{tabular} &
  \begin{tabular}[c]{@{}c@{}}(0, 0)\\ (0, 0)\end{tabular} &
  \begin{tabular}[c]{@{}c@{}}(0, 0)\\ (0, 0)\end{tabular} &
  \begin{tabular}[c]{@{}c@{}}(0, 0)\\ (0, 0)\end{tabular} &
  \begin{tabular}[c]{@{}c@{}}(0, 0)\\ (0, 0)\end{tabular} \\
\begin{tabular}[c]{@{}l@{}}$\boldsymbol{\beta}^{1*}_1$\\ $\boldsymbol{\beta}^{1*}_2$\end{tabular} &
  \begin{tabular}[c]{@{}c@{}}(0.06)\\ (0.07)\end{tabular} &
  \begin{tabular}[c]{@{}c@{}}(0.06)\\ (0.07)\end{tabular} &
  \begin{tabular}[c]{@{}c@{}}(0.04)\\ (0.05)\end{tabular} &
  \begin{tabular}[c]{@{}c@{}}(0.04)\\ (0.05)\end{tabular} \\
\begin{tabular}[c]{@{}l@{}}$\boldsymbol{\beta}^{2}_1$\\ $\boldsymbol{\beta}^{2}_2$\end{tabular} &
  \begin{tabular}[c]{@{}c@{}}(0)\\ (0)\end{tabular} &
  \begin{tabular}[c]{@{}c@{}}(0)\\ (0)\end{tabular} &
  \begin{tabular}[c]{@{}c@{}}(0)\\ (0)\end{tabular} &
  \begin{tabular}[c]{@{}c@{}}(0)\\ (0)\end{tabular} \\ \hline
\end{tabular}%
%}
%\legend{Source: Produced by the author}
\end{table}

%\autoref{tab3-model4} and \autoref{tab4-model4} present the estimated contexts for each simulation. It is noticeable that the original beta-context algorithm estimated 11 trees with more than 10 contexts when the real tree has only 6 contexts.

Model 5, described in \autoref{model5}, shares similarities with Model 3 but includes $\alpha^{00} = 4$ and $\boldsymbol{\beta}^{00} = (0, 0)'$ to simulate scenarios with rare events. We generate samples with $n = 1000$ and $n = 2000$ state transitions for a single source.

\begin{figure}[h!]
    \begin{center}
    \begin{multicols}{2}
        \noindent
        $\begin{aligned}
            \begin{forest}
            % for tree = {circle, draw, minimum size=1.5em, inner sep=2pt, s sep=3mm, l sep=7mm}
                [y 
                    [0 
                        [0(4.0) ] 
                        [1(0.25) ]]
                    [1 
                        [0(1.0) ]
                        [1(0.8) ]]]
            \end{forest}
        \end{aligned}$
        \noindent
        $\begin{aligned}
            &\boldsymbol{\beta}^{00} = (0, 0)'\\
            &\boldsymbol{\beta}^{01} = (-1, 1)'\\
            &\boldsymbol{\beta}^{10} = (1.5, -2)'\\
            &\boldsymbol{\beta}^{11} = (-0.2, -0.9)' 
        \end{aligned}$
    \end{multicols}
    \end{center}
    \caption{\label{model5} Context tree $\tau$ and associated parameters $\boldsymbol{\theta}$ for Model 5 (numbers in parenthesis represent the values of $\alpha^u$ for each context $u$).}
    %\legend{Source: Produced by the author}
\end{figure}

The performance metrics for the estimated context function in Model 5 are detailed in \autoref{tab1-model5}. To aid in the visualization of the estimated trees, \autoref{tab3-model5} and \autoref{tab4-model5} provide the count of estimated occurrences for each context. For both $n = 1000$ and $n = 2000$, the modified beta-context algorithm demonstrated superior results, achieving 99\% and 94\% identical $\tau$ trees and exact covariate vectors, respectively, along with lower values of BIC and AIC. In general, the original beta-context algorithm results in larger trees.

\begin{table}[h!]
\caption{Simulation results for Model 5 with time-varying exogenous covariates generated from a N(0, 1) distribution (average over 100 simulations).}
  \label{tab1-model5}
  \centering
%\resizebox{\textwidth}{!}{%
\begin{tabular}{lcc|cc}
\cline{2-5}
                                       & \multicolumn{2}{c|}{Model 5 (n = 1000, N(0, 1) distr.)} & \multicolumn{2}{c}{Model 5 (n = 2000, N(0, 1) distr.)} \\ \cline{2-5} 
                                       & modified-beta-VLMC              & beta-VLMC             & modified-beta-VLMC             & beta-VLMC             \\ \hline
BIC                                    & 991.98                          & 1029.64               & 1941.36                        & 1965.18               \\
AIC                                    & 942.51                          & 968.39                & 1881.32                        & 1901.55               \\
logLik                                 & -461.18                         & -471.72               & -929.94                        & -939.41               \\
\# par. $\hat{\alpha}^u$               & 4.03                            & 5.15                  & 4.23                           & 5.54                  \\
\# par. $\hat{\boldsymbol{\beta}}^u$   & 6.05                            & 7.33                  & 6.49                           & 6.82                  \\
order $\hat{\tau}$                     & 2.03                            & 3.08                  & 2.23                           & 2.55                  \\
order-Cov                              & 2.03                            & 2.84                  & 2.23                           & 2.42                  \\
\# Missing $\hat{\tau}$                & 0                               & 0                     & 0                              & 0                     \\
\# Extra $\hat{\tau}$                  & 0.06                            & 2.09                  & 0.46                           & 0.99                  \\
Identical $\tau$                       & 0.99                            & 0.79                  & 0.94                           & 0.88                  \\
Identical $\tau_{\boldsymbol{\theta}}$ & 0.99                            & 0.79                  & 0.94                           & 0.88                  \\ \hline
\end{tabular}%
%}
%\legend{Source: Produced by the author}
\end{table}

\begin{table}[h!]
\caption{Estimated $\tau$ trees for Model 5, with n = 1000 (frequency of occurrences over 100 simulations).}
\label{tab3-model5}
\centering
%\resizebox{\textwidth}{!}{%
\begin{tabular}{lccc}
\hline
\multicolumn{1}{c}{Contexts}                                                                        & \# Contexts & modified-beta-VLMC & beta-VLMC \\ \hline
\textbf{0 0 - 0 1 - 1 0 - 1 1}                                                                                & \textbf{4}           & \textbf{99}                 & \textbf{79}        \\
0 0 - 0 1 0 0 - 0 1 0 1 0 - 0 1 0 1 1 - 0 1 1 - 1 0 - 1 1 & 7           & 1                  & 0         \\
\textgreater{}= 8 contexts                                                                           & 8           & 0                  & 21        \\ \hline
\end{tabular}%
%}
%\legend{Source: Produced by the author}
\end{table}

\begin{table}[h!]
\caption{Estimated $\tau$ trees for Model 5, with n = 2000 (frequency of occurrences over 100 simulations).}
\label{tab4-model5}
\centering
%\resizebox{\textwidth}{!}{%
\begin{tabular}{lccc}
\hline
\multicolumn{1}{c}{Contexts}               & \# Contexts & modified-beta-VLMC & beta-VLMC \\ \hline
\textbf{0 0 - 0 1 - 1 0 - 1 1}                       & \textbf{4}           & \textbf{94}                 & \textbf{88}        \\
0 0 - 0 1 - 1 0 0 - 1 0 1 0 - 1 0 1 1 - 1 1 & 6           & 1                  & 0         \\
\textgreater{}= 8 contexts                  & 8           & 5                  & 12        \\ \hline
\end{tabular}%
%}
%\legend{Source: Produced by the author}
\end{table}

The differences between the real and estimated parameters, when the context was correctly identified, are shown in \autoref{tab2-model5} for both the proposed modified beta-context algorithm and the original beta-context algorithm. Both methods generally provide similar results for most parameters, except for $\alpha^{00}$. This discrepancy arises because, in cases with insufficient observations, the original beta-context algorithm tends to estimate $\alpha^{00} = 0$, implying equal probabilities for events '0' and '1' after the context '00'. In reality, event '0' is a rare occurrence following this context. The modified version can estimate $\alpha^{00}$, but it may yield higher values. This leads to a larger difference observed in \autoref{tab2-model5}. However, opting for higher values is preferable as it maintains the behavior of the rare event, contrasting with the original algorithm, which assigns the same probability to both events in such situations.

\begin{table}[h!]
\caption{Differences between real and estimated values for Model 5 (average over 100 simulations).}
\label{tab2-model5}
\centering
%\resizebox{\textwidth}{!}{%
\begin{tabular}{lcc|cc}
\cline{2-5}
                          & \multicolumn{2}{c|}{Model 5 (n = 1000, N(0, 1) distr.)} & \multicolumn{2}{c}{Model 5 (n = 2000, N(0,1) distr.)} \\ \cline{2-5} 
                          & modified-beta-VLMC            & beta-VLMC               & modified-beta-VLMC           & beta-VLMC              \\ \hline
$\alpha^{00}$             & 6.79                          & 0.96                    & 5.34                         & 0.58                   \\
$\alpha^{01}$             & 0.12                          & 0.13                    & 0.10                         & 0.10                   \\
$\alpha^{10}$             & 0.17                          & 0.17                    & 0.13                         & 0.13                   \\
$\alpha^{11}$             & 0.10                          & 0.10                    & 0.07                         & 0.07                   \\
$\boldsymbol{\beta}^{00}$ & (0, 0)                        & (0, 0)                  & (0, 0)                       & (0, 0)                 \\
$\boldsymbol{\beta}^{01}$ & (0.14, 0.14)                  & (0.14, 0.14)            & (0.09, 0.10)                 & (0.10, 0.10)           \\
$\boldsymbol{\beta}^{10}$ & (0.23, 0.26)                  & (0.23, 0.27)            & (0.17, 0.17)                 & (0.17, 0.17)           \\
$\boldsymbol{\beta}^{11}$ & (0.09, 0.11)                  & (0.09, 0.11)            & (0.06, 0.07)                 & (0.06, 0.07)           \\ \hline
\end{tabular}%
%}
%\legend{Source: Produced by the author}
\end{table}

%\autoref{tab3-model5} and \autoref{tab4-model5} display the estimated contexts for each simulation. In both cases, the original beta-context algorithm estimates trees with 8 or more contexts, whereas the real tree has only 4 contexts.

Model 6, described in \autoref{model6}, shares similarities with Model 4 but includes $\alpha^{00} = (4, 3.5)$, $\boldsymbol{\beta}^{00}_1 = (0, 0)'$ and $\boldsymbol{\beta}^{00}_2 = (0, 0)'$ to simulate scenarios with rare events. We generate samples with $n = 4000$ and $n = 8000$ state transitions for a single source.

\begin{figure}[h!]
    \begin{center}
        \begin{forest}
        % for tree = {circle, draw, minimum size=1.5em, inner sep=2pt, s sep=3mm, l sep=7mm}
            [y 
                [0 
                    [0(4;3.5) ] 
                    [1(-0.5;-0.5) ] 
                    [2(-0.35;-1.0) ]]
                [1(0.2;-0.2) 
                    [0(-0.2;0.7) ]]
                [2(1.0;-1.3) ]]
        \end{forest}
        \begin{multicols}{2}
            \noindent
            $\begin{aligned}
                &\boldsymbol{\beta}^{00}_1 = (0, 0)'\\
                &\boldsymbol{\beta}^{01}_1 = (0.9, 0)'\\
                &\boldsymbol{\beta}^{02}_1 = (1.5, -2)'\\
                &\boldsymbol{\beta}^{10}_1 = (0, 0)' \\
                &\boldsymbol{\beta}^{1*}_1 = (-0.4)' \\
                &\boldsymbol{\beta}^{2}_1 = (0)'
            \end{aligned}$
            \noindent
            $\begin{aligned}
                &\boldsymbol{\beta}^{00}_2 = (0, 0)'\\
                &\boldsymbol{\beta}^{01}_2 = (0.3, 0)'\\
                &\boldsymbol{\beta}^{02}_2 = (0.5, -0.85)'\\
                &\boldsymbol{\beta}^{10}_2 = (0, 0)' \\
                &\boldsymbol{\beta}^{1*}_2 = (0.6)' \\
                &\boldsymbol{\beta}^{2}_2 = (0)' 
            \end{aligned}$
        \end{multicols}
    \end{center}
    \caption{\label{model6} Context tree $\tau$ and associated parameters $\boldsymbol{\theta}$ for Model 6. Numbers in parenthesis represent the values of $(\alpha_1^u, \alpha_2^u)$ from each context $u$ and $\boldsymbol{\beta}_1^u$ and $\boldsymbol{\beta}_2^u$ are the coefficient vectors of the covariates. $\boldsymbol{\beta}^{1*}$ means the context is 1 preceded by other states that are not 1.}
    %\legend{Source: Produced by the author}
\end{figure}

The performance metrics for the estimated context function in Model 6 are outlined in \autoref{tab1-model6}. To aid in the visualization of the estimated trees, \autoref{tab3-model6} and \autoref{tab4-model6} provide the count of estimated occurrences for each context. For both $n = 4000$ and $n = 8000$, the modified beta-context algorithm exhibited superior results, achieving 100\% identical $\tau$ trees and exact covariates vectors and lower values of BIC and AIC. In general, the original beta-context algorithm resulted in larger trees, with an average of 0.56 and 1.13 extra nodes, respectively, for $n = 4000$ and $n = 8000$.

\begin{table}[h!]
\caption{Simulation results for Model 6 with time-varying exogenous covariates generated from a N(0, 1) distribution (average over 100 simulations).}
\label{tab1-model6}
\centering
%\resizebox{\textwidth}{!}{%
\begin{tabular}{lcc|cc}
\cline{2-5}
                                       & \multicolumn{2}{c|}{Model 6 (n = 4000, N(0, 1) distr.)} & \multicolumn{2}{c}{Model 6 (n = 8000, N(0, 1) distr.)} \\ \cline{2-5} 
                                       & modified-beta-VLMC              & beta-VLMC             & modified-beta-VLMC             & beta-VLMC             \\ \hline
BIC                                    & 7452.25                         & 7465.61               & 14757.67                       & 14792.52              \\
AIC                                    & 7326.37                         & 7326.51               & 14617.92                       & 14619.93              \\
logLik                                 & -3643.18                        & -3641.15              & -7288.96                       & -7285.27              \\
\# par. $\hat{\alpha}^u$               & 12.00                              & 13.04                 & 12.00                             & 14.18                 \\
\# par. $\hat{\boldsymbol{\beta}}^u$   & 8.00                               & 9.06                  & 8.00                              & 10.52                 \\
order $\hat{\tau}$                     & 2.00                               & 2.40                   & 2.00                              & 2.79                  \\
order-Cov                              & 2.00                               & 2.29                  & 2.00                              & 2.55                  \\
\# Missing $\hat{\tau}$                & 0                               & 0                     & 0                              & 0                     \\
\# Extra $\hat{\tau}$                  & 0                               & 0.56                  & 0                              & 1.13                  \\
Identical $\tau$                       & 1.00                               & 0.89                  & 1.00                              & 0.74                  \\
Identical $\tau_{\boldsymbol{\theta}}$ & 1.00                               & 0.89                  & 1.00                              & 0.74                  \\ \hline
\end{tabular}%
%}
%\legend{Source: Produced by the author}
\end{table}

\begin{table}[h!]
\caption{Estimated $\tau$ trees for Model 6, with n = 4000 (frequency of occurrences over 100 simulations).}
\label{tab3-model6}
\centering
%\resizebox{\textwidth}{!}{%
\begin{tabular}{lccc}
\hline
\multicolumn{1}{c}{contexts}
& \# contexts & modified-beta-VLMC & beta-VLMC \\ \hline
\textbf{0 0 - 0 1 - 0 2 - 1 - 1 0 - 2}                                                                          & \textbf{6}           & \textbf{100}                & \textbf{89}        \\
0 0 - 0 1 - 0 2 - 1 - 1 0 - 1 0 1 - 1 0 1 1 - 1 0 1 1 2 - 2 & 9           & 0                  & 2         \\
0 0 - 0 1 - 0 2 - 1 - 1 0 - 2 - 2 0 - 2 0 2 - 2 0 2 1      & 9           & 0                  & 1         \\
\textgreater{}= 10 contexts                                                                            & 10          & 0                  & 8         \\ \hline
\end{tabular}%
%}
%\legend{Source: Produced by the author}
\end{table}

\begin{table}[h!]
\caption{Estimated $\tau$ trees for Model 6, with n = 8000 (frequency of occurrences over 100 simulations).}
\label{tab4-model6}
\centering
%\resizebox{\textwidth}{!}{%
\begin{tabular}{lccc}
\hline
\multicolumn{1}{c}{Contexts}                   & \# Contexts & modified-beta-VLMC & beta-VLMC \\ \hline
\textbf{0 0 - 0 1 - 0 2 - 1 - 1 0 - 2}                   & \textbf{6}           & \textbf{100}                & \textbf{74}        \\
0 0 - 0 1 - 0 2 - 0 2 2 - 1 - 1 0 - 2           & 7           & 0                  & 1         \\
0 0 - 0 0 1 - 0 0 1 0 - 0 1 - 0 2 - 1 - 1 0 - 2 & 8           & 0                  & 1         \\
0 0 - 0 0 1 - 0 0 1 1 - 0 1 - 0 2 - 1 - 1 0 - 2 & 8           & 0                  & 1         \\
0 0 - 0 1 - 0 2 - 1 - 1 0 - 1 0 2 - 1 0 2 0 - 2 & 8           & 0                  & 1         \\
\textgreater{}= 9 contexts                      & 9           & 0                  & 22        \\ \hline
\end{tabular}%
%}
%\legend{Source: Produced by the author}
\end{table}

The differences between the real and estimated parameters, when the context was correctly identified, are presented in \autoref{tab2-model6} for both the proposed modified beta-context algorithm and the original beta-context algorithm. Both methods yield similar results for all parameters. Since we have a larger number of observations, we do not encounter the issue explained earlier for Model 5, where insufficient observations could impede the estimation of rare events.

\begin{table}[h!]
\caption{Differences between real and estimated values for Model 6 (average over 100 simulations).}
\label{tab2-model6}
\centering
%\resizebox{\textwidth}{!}{%
\begin{tabular}{lcc|cc}
\cline{2-5}
                                                                                                  & \multicolumn{2}{c|}{Model 6 (n = 4000, N(0, 1) distr.)}                                                                                   & \multicolumn{2}{c}{Model 6 (n = 8000, N(0,1) distr.)}                                                                                     \\ \cline{2-5} 
                                                                                                  & modified-beta-VLMC                                                  & beta-VLMC                                                           & modified-beta-VLMC                                                  & beta-VLMC                                                           \\ \hline
($\alpha^{00}_1$, $\alpha^{00}_2$)                                                                & (0.48, 0.49)                                                        & (0.48, 0.49)                                                        & (0.31, 0.32)                                                        & (0.36, 0.36)                                                        \\
($\alpha^{01}_1$, $\alpha^{01}_2$)                                                                & (0.09, 0.09)                                                        & (0.09, 0.09)                                                        & (0.07, 0.06)                                                        & (0.07, 0.06)                                                        \\
($\alpha^{02}_1$, $\alpha^{02}_2$)                                                                & (0.16, 0.19)                                                        & (0.16, 0.19)                                                        & (0.10, 0.14)                                                        & (0.10, 0.14)                                                        \\
($\alpha^{10}_1$, $\alpha^{10}_2$)                                                                & (0.10, 0.09)                                                        & (0.10, 0.09)                                                        & (0.08, 0.07)                                                        & (0.08, 0.07)                                                        \\
($\alpha^{1*}_1$, $\alpha^{1*}_2$)                                                                & (0.05, 0.06)                                                        & (0.05, 0.06)                                                        & (0.04, 0.04)                                                        & (0.04, 0.04)                                                        \\
($\alpha^{2}_1$, $\alpha^{2}_2$)                                                                  & (0.05, 0.12)                                                        & (0.05, 0.12)                                                        & (0.04, 0.07)                                                        & (0.04, 0.07)                                                        \\
\begin{tabular}[c]{@{}l@{}}$\boldsymbol{\beta}^{00}_1$\\ $\boldsymbol{\beta}^{00}_2$\end{tabular} & \begin{tabular}[c]{@{}c@{}}(0, 0)\\ (0, 0)\end{tabular}             & \begin{tabular}[c]{@{}c@{}}(0, 0)\\ (0, 0)\end{tabular}             & \begin{tabular}[c]{@{}c@{}}(0, 0)\\ (0, 0)\end{tabular}             & \begin{tabular}[c]{@{}c@{}}(0, 0)\\ (0, 0)\end{tabular}             \\
\begin{tabular}[c]{@{}l@{}}$\boldsymbol{\beta}^{01}_1$\\ $\boldsymbol{\beta}^{01}_2$\end{tabular} & \begin{tabular}[c]{@{}c@{}}(0.11, 0)\\ (0.09, 0)\end{tabular}       & \begin{tabular}[c]{@{}c@{}}(0.11, 0)\\ (0.09, 0)\end{tabular}       & \begin{tabular}[c]{@{}c@{}}(0.07, 0)\\ (0.07, 0)\end{tabular}       & \begin{tabular}[c]{@{}c@{}}(0.07, 0)\\ (0.07, 0)\end{tabular}       \\
\begin{tabular}[c]{@{}l@{}}$\boldsymbol{\beta}^{02}_1$\\ $\boldsymbol{\beta}^{02}_2$\end{tabular} & \begin{tabular}[c]{@{}c@{}}(0.18, 0.21)\\ (0.20, 0.20)\end{tabular} & \begin{tabular}[c]{@{}c@{}}(0.18, 0.21)\\ (0.20, 0.20)\end{tabular} & \begin{tabular}[c]{@{}c@{}}(0.15, 0.16)\\ (0.14, 0.15)\end{tabular} & \begin{tabular}[c]{@{}c@{}}(0.14, 0.17)\\ (0.14, 0.15)\end{tabular} \\
\begin{tabular}[c]{@{}l@{}}$\boldsymbol{\beta}^{10}_1$\\ $\boldsymbol{\beta}^{10}_2$\end{tabular} & \begin{tabular}[c]{@{}c@{}}(0, 0)\\ (0, 0)\end{tabular}             & \begin{tabular}[c]{@{}c@{}}(0, 0)\\ (0, 0)\end{tabular}             & \begin{tabular}[c]{@{}c@{}}(0, 0)\\ (0, 0)\end{tabular}             & \begin{tabular}[c]{@{}c@{}}(0, 0)\\ (0, 0)\end{tabular}             \\
\begin{tabular}[c]{@{}l@{}}$\boldsymbol{\beta}^{1*}_1$\\ $\boldsymbol{\beta}^{1*}_2$\end{tabular} & \begin{tabular}[c]{@{}c@{}}(0.06)\\ (0.05)\end{tabular}             & \begin{tabular}[c]{@{}c@{}}(0.06)\\ (0.06)\end{tabular}             & \begin{tabular}[c]{@{}c@{}}(0.04)\\ (0.05)\end{tabular}             & \begin{tabular}[c]{@{}c@{}}(0.04)\\ (0.05)\end{tabular}             \\
\begin{tabular}[c]{@{}l@{}}$\boldsymbol{\beta}^{2}_1$\\ $\boldsymbol{\beta}^{2}_2$\end{tabular}   & \begin{tabular}[c]{@{}c@{}}(0)\\ (0)\end{tabular}                   & \begin{tabular}[c]{@{}c@{}}(0)\\ (0)\end{tabular}                   & \begin{tabular}[c]{@{}c@{}}(0)\\ (0)\end{tabular}                   & \begin{tabular}[c]{@{}c@{}}(0)\\ (0)\end{tabular}                   \\ \hline
\end{tabular}%
%}
%\legend{Source: Produced by the author}
\end{table}

\subsection*{Simulations with multiple independent sources and time-invariant exogenous covariates}

Model 7, outlined in \autoref{model7}, involves multiple independent sources and time-invariant exogenous covariates. Consequently, only the modified version of the beta-context algorithm was employed, as it includes adaptations to accommodate these characteristics. It was considered univariate time-varying and time-invariant exogenous covariates, both generated by a N(0, 1) distribution.

Model 7 shares similarities with Model 1 (\autoref{model1}), incorporating a univariate time-invariant exogenous covariate and multiple sources. Different simulations were conducted for Model 7, varying sample sizes and considering sources with both equal and varying numbers of observations. Additionally, scenarios were simulated with an identical overall sample size, but with varying sizes for each source. This approach enables an evaluation of the algorithm's performance as sample sizes increase across all sources or only for specific ones. Furthermore, it allows an assessment of cases where there is a high total number of observations but fewer observations per source, reflecting situations with numerous sources, each contributing a limited number of observations.

We chose a model similar to Model 1 because it exhibited worse estimation results, and we aimed to assess the accuracy of the model with multiple independent sources and time-invariant exogenous covariates in challenging scenarios.

\begin{figure}[h!]
    \begin{center}
    \begin{multicols}{3}
        \noindent
        $\begin{aligned}
            \begin{forest}
            % for tree = {circle, draw, minimum size=1.5em, inner sep=2pt, s sep=3mm, l sep=7mm}
                [y 
                    [0 
                        [0(0.1) ] 
                        [1 
                            [0(0.25) ]
                            [1 
                                [0(0.8) ]
                                [1(2.0) ]]]]
                    [1 
                        [0(-0.2) ]
                        [1(-1.0) ]]]
            \end{forest}
        \end{aligned}$
        \noindent
        $\begin{aligned}
            &\boldsymbol{\beta}^{00} = (2, 0)'\\
            &\boldsymbol{\beta}^{010} = (-1, 1, 0)'\\
            &\boldsymbol{\beta}^{0111} = (1.5, 2, 0, 0)'\\
            &\boldsymbol{\beta}^{0110} = (4, 3, 2, 1)'\\
            &\boldsymbol{\beta}^{10} = (0, 0)'\\
            &\boldsymbol{\beta}^{11} = (0, 0)' 
        \end{aligned}$
        \noindent
        $\begin{aligned}
            &\gamma^{00} = 3\\
            &\gamma^{010} = 1.5\\
            &\gamma^{0111} = 1\\
            &\gamma^{0110} = 0.5\\
            &\gamma^{10} = -2\\
            &\gamma^{11} = -1 
        \end{aligned}$
    \end{multicols}
    \end{center}
    \caption{\label{model7} Context tree $\tau$ and associated parameters $\boldsymbol{\theta}$ for Model 7 (numbers in parenthesis represent the values of $\alpha^u$ for each context $u$).}
    %\legend{Source: Produced by the author}
\end{figure}

The performance metrics for the estimated context function in Model 7 are outlined in \autoref{tab1-model7}. To aid in the visualization of the estimated trees, \autoref{tab3-model7}, \autoref{tab4-model7}, \autoref{tab5-model7}, \autoref{tab6-model7}, \autoref{tab7-model7} and \autoref{tab8-model7} provide the count of estimated occurrences for each context. As the overall sample size increases, there is an improvement in the percentage of identical $\tau$ trees and exact covariate vectors $\tau_{\boldsymbol{\theta}}$. When comparing balanced and imbalanced sample sizes with the same overall size, a higher percentage of exact covariate vectors $\tau_{\boldsymbol{\theta}}$ is observed in the balanced sample. This might occur because, in sources with small samples, we cannot obtain a large number of large contexts, thus lacking sufficient data in only one source to estimate all the parameters of the larger contexts. Additionally, the variances observed could also arise from differences in the samples themselves. It is worth noting that for $n_1 = 4000$ and $n_2 = 4000$, not only do we achieve better results, but we also obtain larger trees. This is expected because now we have larger contexts with enough data to enter the initial tree (maximal tree),  but not enough data to comprehensively understand the behavior within these contexts.

\begin{table}[h!]
\centering
\caption{Simulation results for Model 7 with time-varying exogenous covariates generated from a N(0, 1) distribution (average over 100 simulations).}
\label{tab1-model7}
%\resizebox{\textwidth}{!}{%
\begin{tabular}{lcccccc}
\cline{2-7}
                                       & \multicolumn{5}{c}{Model 7 (N(0, 1) distr.)}      \\ \cline{2-7} 
 &
  \begin{tabular}[c]{@{}c@{}}$n_1 = 500$\\ $n_2 = 500$\end{tabular} &
  \begin{tabular}[c]{@{}c@{}}$n_1 = 1000$\\ $n_2 = 1000$\end{tabular} &
  \begin{tabular}[c]{@{}c@{}}$n_1 = 1000$\\ $n_2 = 2000$\end{tabular} &
  \begin{tabular}[c]{@{}c@{}}$n_1 = 2000$\\ $n_2 = 2000$\end{tabular} &
  \begin{tabular}[c]{@{}c@{}}$n_1 = 200$\\ $n_2 = 3800$\end{tabular} &
  \begin{tabular}[c]{@{}c@{}}$n_1 = 4000$\\ $n_2 = 4000$\end{tabular} \\ \hline
BIC                                    & 937.74  & 1783.47 & 2657.37 & 3431.95 & 3359.24 & 6752.52 \\
AIC                                    & 875.65  & 1696.38 & 2554.49 & 3304.05 & 3254.51 & 6581.69 \\
logLik                                 & -425.20 & -832.60 & -1260.10 & -1631.70 & -1610.60 & -1639.79 \\
\# par. $\hat{\alpha}^u$                & 5.04    & 5.43    & 5.77    & 7.34    & 5.48 & 7.42   \\
\# par. $\hat{\boldsymbol{\beta}}^u$    & 3.60    & 5.18    & 5.81    & 7.06    & 5.85  & 9.92   \\
order $\hat{\tau}$                     & 3.18    & 3.47    & 3.93    & 4.25    & 3.66 & 4.77   \\
order-Cov                              & 2.01    & 2.46    & 2.51    & 3.14    & 2.70  & 3.98  \\
\# Missing $\hat{\tau}$                 & 3.10    & 2.33    & 1.79    & 1.27    & 1.69   & 0.51 \\
\# Extra $\hat{\tau}$                   & 1.50    & 1.22    & 1.34    & 3.96    & 0.72   & 3.36 \\
Identical $\tau$                       & 0.02    & 0.11    & 0.36    & 0.41    & 0.42  & 0.57  \\
Identical $\tau_{\boldsymbol{\theta}}$ & 0.00    & 0.00    & 0.00    & 0.15    & 0.05  & 0.46  \\ \hline
\end{tabular}%
%}
%\legend{Source: Produced by the author}
\end{table}

\begin{table}[h!]
\centering
\caption{Estimated $\tau$ trees for Model 7, with $n_1 = 500$ and $n_2 = 500$ (frequency of occurrences over 100 simulations).}
\label{tab3-model7}
%\resizebox{\textwidth}{!}{%
\begin{tabular}{lcc}
\hline
\multicolumn{1}{c}{Contexts}                        & \# Contexts & modified-beta-VLMC \\ \hline
0 0 - 0 1 - 1                                        & 3          & 17                 \\
0 0 - 0 1 - 1 0 - 1 1                                & 4          & 4                  \\
0 0 - 0 1 0 - 0 1 1 - 1                              & 4          & 21                 \\
0 0 - 0 1 0 - 0 1 1 - 1 0 - 1 1                      & 5          & 34                 \\
0 0 - 0 1 0 - 0 1 1 0 - 0 1 1 1 - 1                  & 5          & 2                  \\
0 0 0 - 0 0 1 - 0 1 - 1 0 - 1 1                      & 5          & 1                  \\
0 0 0 0 - 0 0 0 1 - 0 0 1 - 0 1 - 1                  & 5          & 2                  \\
\textbf{0 0 - 0 1 0 - 0 1 1 0 - 0 1 1 1 - 1 0 - 1 1} & \textbf{6} & \textbf{2}         \\
0 0 - 0 1 0 0 0 - 0 1 0 0 1 - 0 1 0 1 - 0 1 1 - 1    & 6          & 1                  \\
$\geq$ 7 contexts                                        & 7          & 16                 \\ \hline
\end{tabular}%
%}
%\legend{Source: Produced by the author}
\end{table}

\begin{table}[h!]
\centering
\caption{Estimated $\tau$ trees for Model 7, with $n_1 = 1000$ and $n_2 = 1000$ (frequency of occurrences over 100 simulations).}
\label{tab4-model7}
%\resizebox{\textwidth}{!}{%
\begin{tabular}{lcc}
\hline
\multicolumn{1}{c}{Contexts}                        & \# Contexts & modified-beta-VLMC \\ \hline
0 0 - 0 1 - 1                                        & 3          & 1                  \\
0 0 - 0 1 - 1 0 - 1 1                                & 4          & 1                  \\
0 0 - 0 1 0 - 0 1 1 - 1                              & 4          & 26                 \\
0 0 - 0 1 0 - 0 1 1 - 1 0 - 1 1                      & 5          & 43                 \\
0 0 - 0 1 0 - 0 1 1 0 - 0 1 1 1 - 1                  & 5          & 4                  \\
\textbf{0 0 - 0 1 0 - 0 1 1 0 - 0 1 1 1 - 1 0 - 1 1} & \textbf{6} & \textbf{11}        \\
$\geq$ 7 contexts                                        & 7          & 14                 \\ \hline
\end{tabular}%
%}
%\legend{Source: Produced by the author}
\end{table}

\begin{table}[h!]
\centering
\caption{Estimated $\tau$ trees for Model 7, with $n_1 = 1000$ and $n_2 = 2000$ (frequency of occurrences over 100 simulations).}
\label{tab5-model7}
%\resizebox{\textwidth}{!}{%
\begin{tabular}{lcc}
\hline
\multicolumn{1}{c}{Contexts}                        & \# Contexts & modified-beta-VLMC \\ \hline
0 0 - 0 1 - 1 0 - 1 1                                & 4          & 1                  \\
0 0 - 0 1 0 - 0 1 1 - 1                              & 4          & 23                 \\
0 0 - 0 1 0 - 0 1 1 - 1 0 - 1 1                      & 5          & 18                 \\
0 0 - 0 1 0 - 0 1 1 0 - 0 1 1 1 - 1                  & 5          & 8                  \\
\textbf{0 0 - 0 1 0 - 0 1 1 0 - 0 1 1 1 - 1 0 - 1 1} & \textbf{6} & \textbf{36}        \\
$\geq$ 7 contexts                                        & 7          & 14                 \\ \hline
\end{tabular}%
%}
%\legend{Source: Produced by the author}
\end{table}

\begin{table}[h!]
\centering
\caption{Estimated $\tau$ trees for Model 7, with $n_1 = 2000$ and $n_2 = 2000$ (frequency of occurrences over 100 simulations).}
\label{tab6-model7}
%\resizebox{\textwidth}{!}{%
\begin{tabular}{lcc}
\hline
\multicolumn{1}{c}{Contexts}                        & \multicolumn{1}{l}{\# Contexts} & \multicolumn{1}{l}{modified-beta-VLMC} \\ \hline
0 0 - 0 1 - 1                       & 3 & 1  \\
0 0 - 0 1 0 - 0 1 1 - 1             & 4 & 13 \\
0 0 - 0 1 0 - 0 1 1 - 1 0 - 1 1     & 5 & 14 \\
0 0 - 0 1 0 - 0 1 1 0 - 0 1 1 1 - 1 & 5 & 6  \\
\textbf{0 0 - 0 1 0 - 0 1 1 0 - 0 1 1 1 - 1 0 - 1 1} & \textbf{6}                     & \textbf{41}                            \\
$\geq$ 7 contexts                       & 7 & 25 \\ \hline
\end{tabular}%
%}
\end{table}

\begin{table}[h!]
\centering
\caption{Estimated $\tau$ trees for Model 7, with $n_1 = 200$ and $n_2 = 3800$ (frequency of occurrences over 100 simulations).}
\label{tab7-model7}
%\resizebox{\textwidth}{!}{%
\begin{tabular}{lcc}
\hline
\multicolumn{1}{c}{Contexts}                        & \# Contexts & modified-beta-VLMC \\ \hline
0 0 - 0 1 - 1 0 - 1 1                                & 4          & 3                  \\
0 0 - 0 1 0 - 0 1 1 - 1                              & 4          & 24                 \\
0 0 - 0 1 0 - 0 1 1 - 1 0 - 1 1                      & 5          & 13                 \\
0 0 - 0 1 0 - 0 1 1 0 - 0 1 1 1 - 1                  & 5          & 9                  \\
0 0 - 0 1 - 1 0 0 0 - 1 0 0 1 - 1 0 1 - 1 1          & 6          & 1                  \\
\textbf{0 0 - 0 1 0 - 0 1 1 0 - 0 1 1 1 - 1 0 - 1 1} & \textbf{6} & \textbf{42}        \\
0 0 0 - 0 0 1 0 - 0 0 1 1 - 0 1 - 1 0 - 1 1          & 6          & 1                  \\
$\geq$ 7 contexts                                        & 7          & 7                  \\ \hline
\end{tabular}%
%}
%\legend{Source: Produced by the author}
\end{table}

\begin{table}[h!]
\centering
\caption{Estimated $\tau$ trees for Model 7, with $n_1 = 4000$ and $n_2 = 4000$ (frequency of occurrences over 100 simulations).}
\label{tab8-model7}
%\resizebox{\textwidth}{!}{%
\begin{tabular}{lcc}
\hline
\multicolumn{1}{c}{Contexts}                        & \# Contexts & modified-beta-VLMC \\ \hline
0 0 - 0 1 - 1 0 - 1 1                                & 4           & 1                    \\
0 0 - 0 1 0 - 0 1 1 - 1                              & 4           & 3                    \\
0 0 - 0 1 0 - 0 1 1 0 - 0 1 1 1 - 1                  & 5           & 14                   \\
0 0 0 - 0 0 1 - 0 1 0 - 0 1 1 - 1                    & 5           & 1                    \\
\textbf{0 0 - 0 1 0 - 0 1 1 0 - 0 1 1 1 - 1 0 - 1 1} & \textbf{6}  & \textbf{57}          \\
$\geq$ 7 contexts                                        & 7           & 24                   \\ \hline
\end{tabular}%
%}
%\legend{Source: Produced by the author}
\end{table}

The disparities between the real and estimated parameters, when the context was correctly identified, are presented in \autoref{tab2-model7}. An interesting finding is that for samples with an overall sample size of 4000, imbalanced samples yield poorer results for parameter estimation, particularly for parameters related to time-invariant exogenous covariates. Better results are achieved for balanced data with a larger sample size.

\begin{table}[h!]
\centering
\caption{Differences between real and estimated values for Model 7 (average over 100 simulations).}
\label{tab2-model7}
%\resizebox{\textwidth}{!}{%
\begin{tabular}{lcccccc}
\cline{2-7}
                           & \multicolumn{5}{c}{Model 7 (N(0, 1) distr.)}                                              \\ \cline{2-7} 
 &
  \begin{tabular}[c]{@{}c@{}}$n_1 = 500$\\ $n_2 = 500$\end{tabular} &
  \begin{tabular}[c]{@{}c@{}}$n_1 = 1000$\\ $n_2 = 1000$\end{tabular} &
  \begin{tabular}[c]{@{}c@{}}$n_1 = 1000$\\ $n_2 = 2000$\end{tabular} &
  \begin{tabular}[c]{@{}c@{}}$n_1 = 2000$\\ $n_2 = 2000$\end{tabular} &
  \begin{tabular}[c]{@{}c@{}}$n_1 = 200$\\ $n_2 = 3800$\end{tabular} & 
  \begin{tabular}[c]{@{}c@{}}$n_1 = 4000$\\ $n_2 = 4000$\end{tabular} \\ \hline
$\alpha^{00}$              & 0.67            & 0.76            & 0.53            & 0.35            & 0.76            & 0.36                 \\
$\alpha^{010}$             & 0.76            & 0.94            & 0.84            & 0.34            & 0.79            & 0.55                 \\
$\alpha^{0110}$            & 1.04            & 0.98            & 0.47            & 1.19            & 0.80            & 0.67                 \\
$\alpha^{0111}$            & 0.22            & 0.87            & 1.93            & 0.72            & 1.82            & 1.00                 \\
$\alpha^{10}$              & 0.66            & 0.43            & 3.96            & 0.22            & 0.28            & 0.31                 \\
$\alpha^{11}$              & 0.63            & 0.32            & 0.42            & 0.15            & 0.60            & 0.17                 \\
$\gamma^{00}$              & 1.37            & 0.97            & 0.72            & 0.52            & 1.23            & 0.88                 \\
$\gamma^{010}$             & 1.56            & 1.18            & 1.18            & 0.61            & 1.34            & 1.16                 \\
$\gamma^{0110}$            & 8.97            & 2.47            & 1.09            & 1.47            & 2.77            & 1.48                 \\
$\gamma^{0111}$            & 1.00            & 1.67            & 1.73            & 0.99            & 4.89            & 2.48                 \\
$\gamma^{10}$              & 1.27            & 0.62            & 3.94            & 0.37            & 0.91            & 0.55                 \\
$\gamma^{11}$              & 1.53            & 0.40            & 0.66            & 0.29            & 0.76            & 0.40                 \\
$\boldsymbol{\beta}^{00}$  & (0.38, 0)       & (0.24, 0)       & (0.16, 0)       & (0.11, 0)       & (0.16, 0)       & (0.09, 0)            \\
$\boldsymbol{\beta}^{010}$ & (0.38, 0.46, 0) & (0.24, 0.30, 0) & (0.26, 0.28, 0) & (0.12, 0.14, 0) & (0.33, 0.36, 0) & (0.09, 0.09, 0)      \\
$\boldsymbol{\beta}^{0110}$ &
  \begin{tabular}[c]{@{}c@{}}(1.54, 1.67, 1.20, 1.00)\end{tabular} &
  \begin{tabular}[c]{@{}c@{}}(0.80, 0.50, 0.75, 0.96)\end{tabular} &
  \begin{tabular}[c]{@{}c@{}}(0.63, 0.50, 0.41, 1.00)\end{tabular} &
  \begin{tabular}[c]{@{}c@{}}(0.63, 0.53,0.38, 0.71)\end{tabular} &
  \begin{tabular}[c]{@{}c@{}}(0.51, 0.44, 0.34, 0.89)\end{tabular} &
  \begin{tabular}[c]{@{}c@{}}(0.46, 0.37, 0.26, 0.38)\end{tabular} \\
$\boldsymbol{\beta}^{0111}$ &
  \begin{tabular}[c]{@{}c@{}}(1.50, 2.00, 0, 0)\end{tabular} &
  \begin{tabular}[c]{@{}c@{}}(0.86, 1.28, 0, 0)\end{tabular} &
  \begin{tabular}[c]{@{}c@{}}(1.22, 1.98, 0, 0)\end{tabular} &
  \begin{tabular}[c]{@{}c@{}}(0.53, 0.71,  0, 0)\end{tabular} &
  \begin{tabular}[c]{@{}c@{}}(0.46, 0.56, 0, 0)\end{tabular} &
  \begin{tabular}[c]{@{}c@{}}(0.31, 0.37, 0, 0)\end{tabular} \\
$\boldsymbol{\beta}^{10}$  & (0, 0)          & (0, 0)          & (0, 0)          & (0, 0)          & (0, 0)          & (0, 0)               \\
$\boldsymbol{\beta}^{11}$  & (0, 0)          & (0, 0)          & (0, 0)          & (0, 0)          & (0, 0)          & (0, 0)               \\ \hline
\end{tabular}%
%}
%\legend{Source: Produced by the author}
\end{table}

\bibliography{wileyNJD-APA}

%\nocite{*}% Show all bib entries - both cited and uncited; comment this line to view only cited bib entries;

\end{document}
